# Supplementary material for: DeepTest Tool Competition 2026: Benchmarking an LLM-Based Automotive Assistant
Source: arXiv:2604.12615 source file (2026-04-14)
Supplement: Supplementary file 1 [file appendix.tex]

\appendix
\section{Additional Results}
Here we include supplementary tables and figures. (internal or repo)

\begin{figure}[p]
    \centering
    % Row 1: Run 1 and Run 2
    \begin{subfigure}[b]{0.46\linewidth}
        \centering
     \includegraphics[width=\linewidth, trim=0 65 0 10, clip]{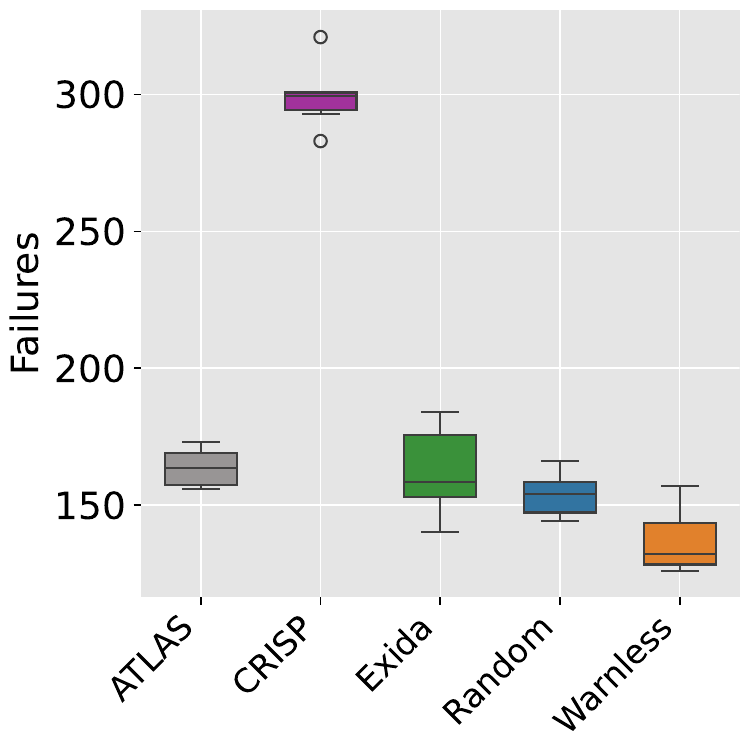}
     \label{fig:sub1}
    \end{subfigure}%
    \hspace{0.02\linewidth} % small horizontal space between figures
    \begin{subfigure}[b]{0.46\linewidth}
        \centering
     \includegraphics[width=\linewidth, trim=0 65 0 10, clip]{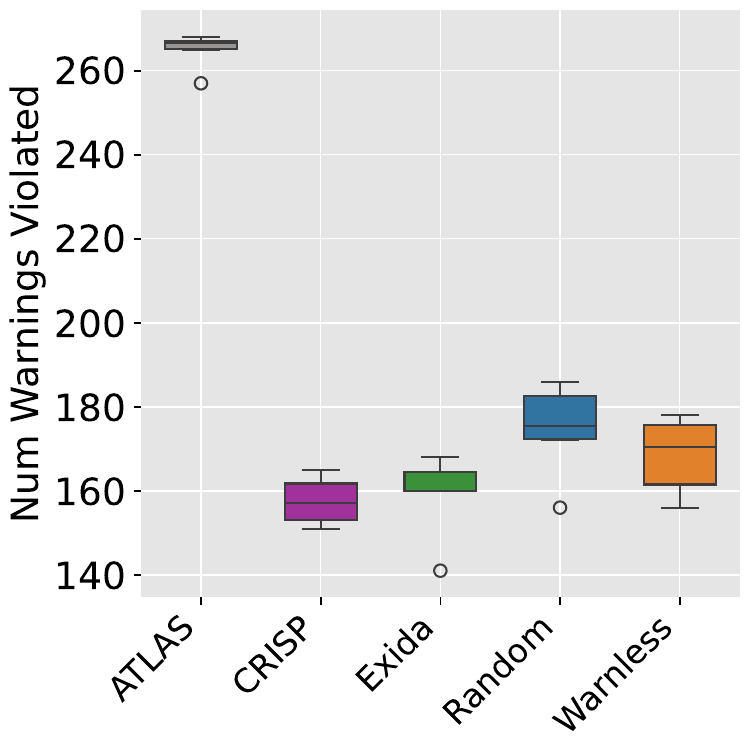}          \label{fig:sub2}
    \end{subfigure}

    \vspace{0.3cm}  % vertical space between rows

    % Row 2: Run 3 and Run 4
    \begin{subfigure}[b]{0.46\linewidth}
        \centering
        \includegraphics[width=\linewidth, trim=0 0 0 10, clip]{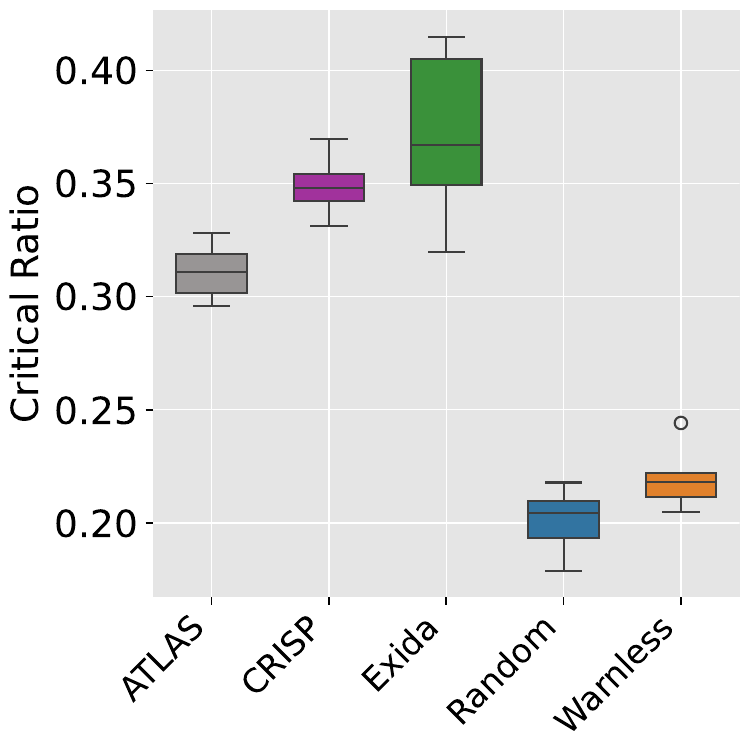}        \label{fig:sub3}
    \end{subfigure}%
    \hspace{0.02\linewidth}
    \begin{subfigure}[b]{0.46\linewidth}
        \centering
     \includegraphics[width=\linewidth, trim=0 0 0 4, clip]{results/gpt4o-mini/initial/coverage_boxplot.pdf}          \label{fig:sub4}
    \end{subfigure}
    \caption{Metric results \suttwo with manual \manualone and LLM \gptfouromini.}
    \label{fig:boxplots-results}
\end{figure}

\begin{figure}[p]
    \centering
    % Row 1: Run 1 and Run 2
    \begin{subfigure}[b]{0.46\linewidth}
        \centering
     \includegraphics[width=\linewidth, trim=0 65 0 10, clip]{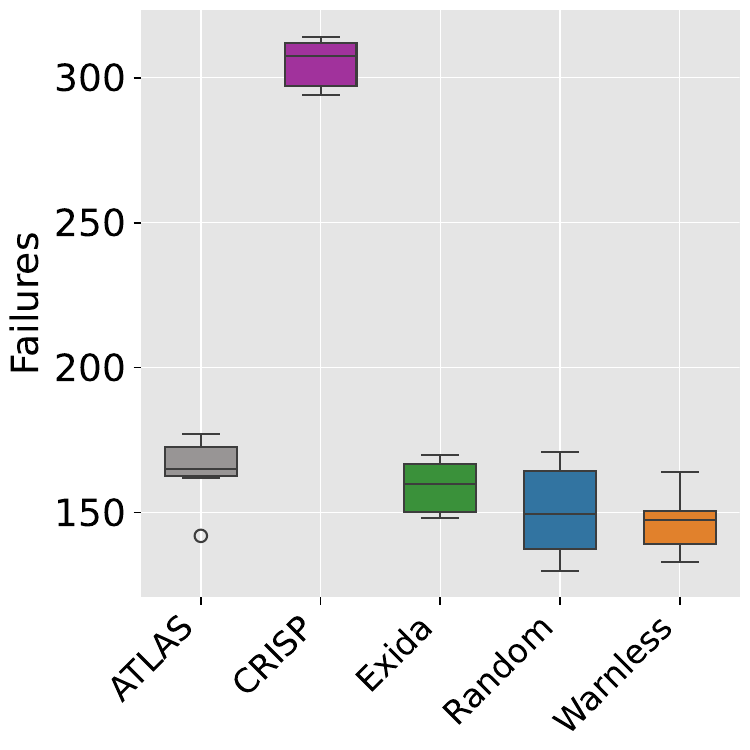}
     \label{fig:sub1}
    \end{subfigure}%
    \hspace{0.02\linewidth} % small horizontal space between figures
    \begin{subfigure}[b]{0.46\linewidth}
        \centering
     \includegraphics[width=\linewidth, trim=0 65 0 10, clip]{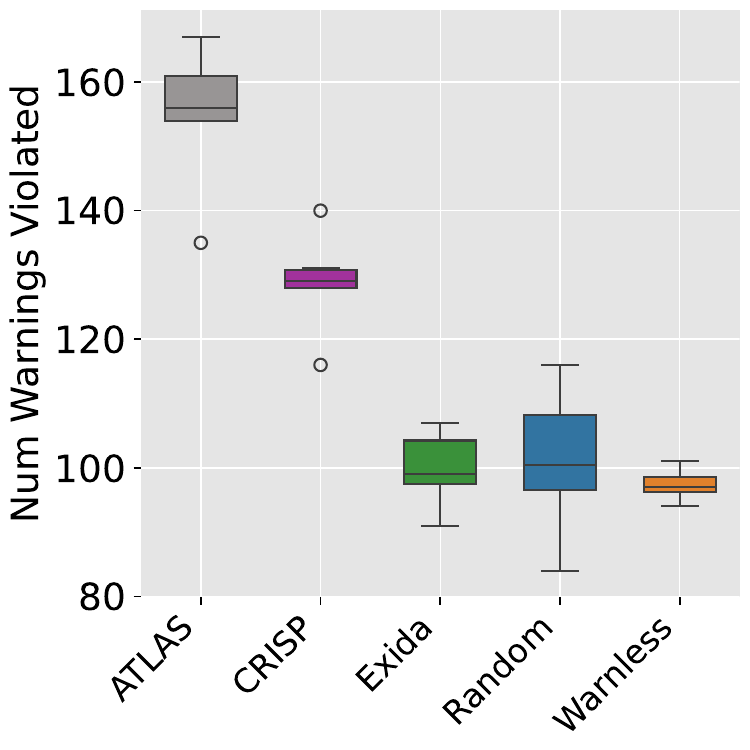}          \label{fig:sub2}
    \end{subfigure}

    \vspace{0.3cm}  % vertical space between rows

    % Row 2: Run 3 and Run 4
    \begin{subfigure}[b]{0.46\linewidth}
        \centering
        \includegraphics[width=\linewidth, trim=0 0 0 10, clip]{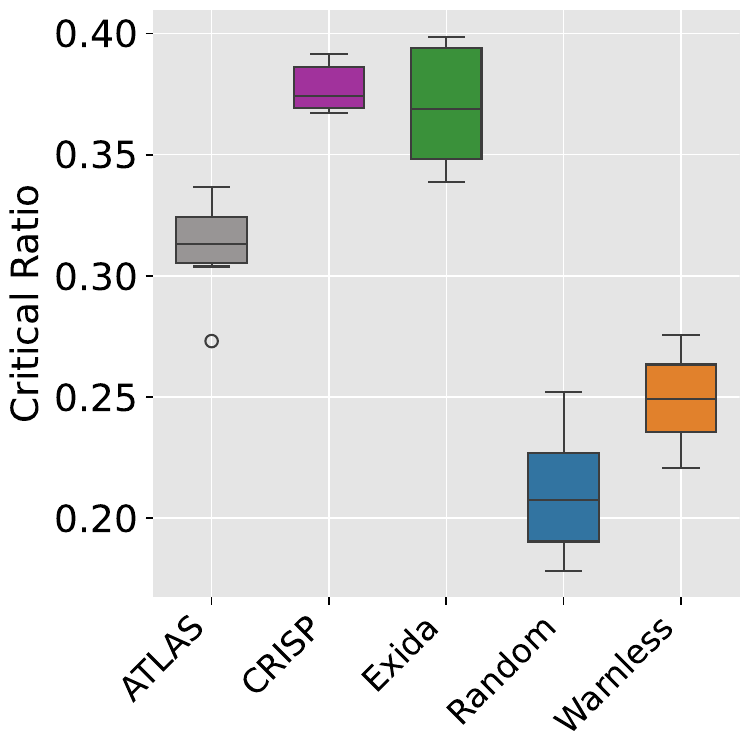}        \label{fig:sub3}
    \end{subfigure}%
    \hspace{0.02\linewidth}
    \begin{subfigure}[b]{0.46\linewidth}
        \centering
     \includegraphics[width=\linewidth, trim=0 0 0 4, clip]{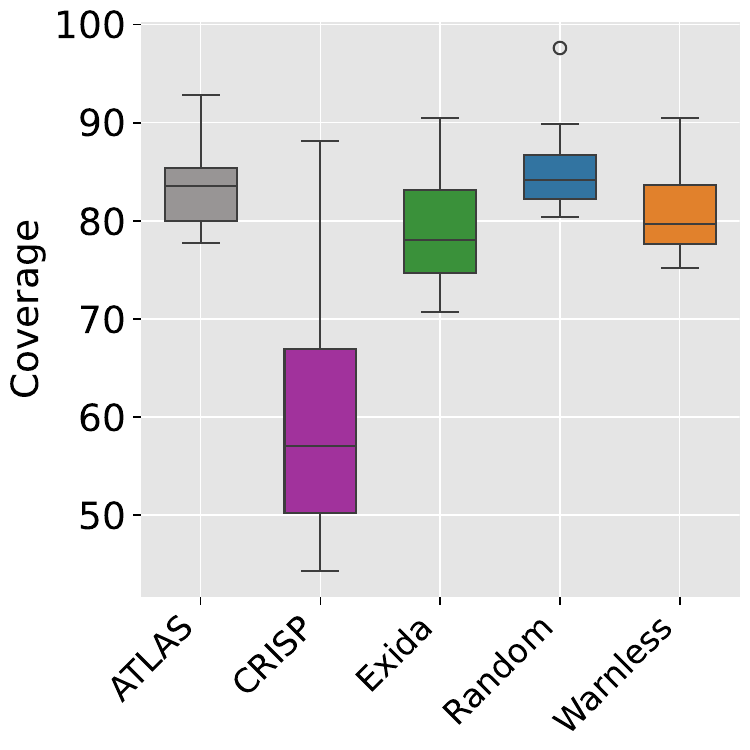}          \label{fig:sub4}
    \end{subfigure}
    \caption{Metric results \suttwo with manual \manualtwo and LLM \gptfivechat.}
    \label{fig:boxplots-results}
\end{figure}

\begin{figure}[p]
    \centering
    % Row 1: Run 1 and Run 2
    \begin{subfigure}[b]{0.46\linewidth}
        \centering
     \includegraphics[width=\linewidth, trim=0 65 0 10, clip]{results/gpt-5-chat/initial/failures_boxplots.pdf}
     \label{fig:sub1}
    \end{subfigure}%
    \hspace{0.02\linewidth} % small horizontal space between figures
    \begin{subfigure}[b]{0.46\linewidth}
        \centering
     \includegraphics[width=\linewidth, trim=0 65 0 10, clip]{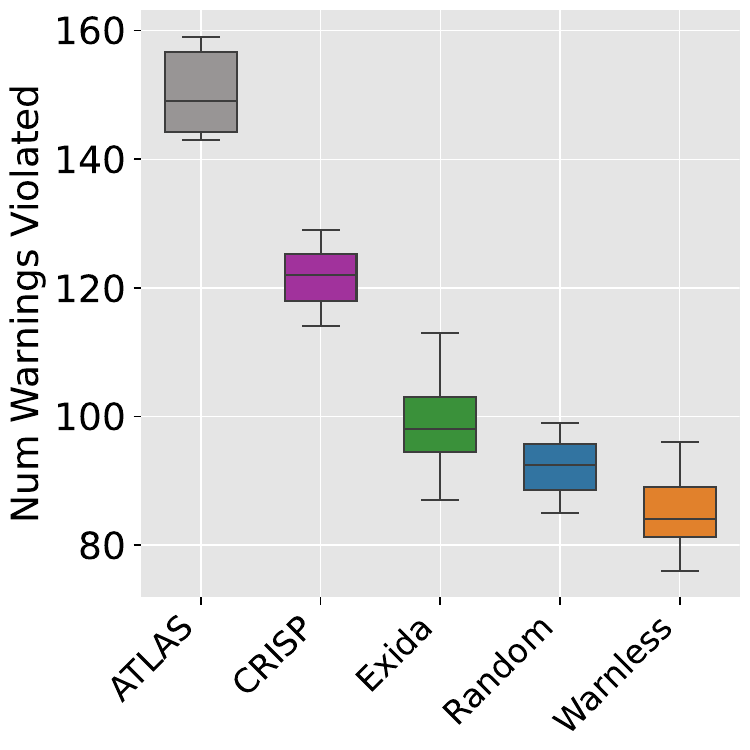}          \label{fig:sub2}
    \end{subfigure}

    \vspace{0.3cm}  % vertical space between rows

    % Row 2: Run 3 and Run 4
    \begin{subfigure}[b]{0.46\linewidth}
        \centering
        \includegraphics[width=\linewidth, trim=0 0 0 10, clip]{results/gpt-5-chat/initial/critical_ratio_boxplots.pdf}        \label{fig:sub3}
    \end{subfigure}%
    \hspace{0.02\linewidth}
    \begin{subfigure}[b]{0.46\linewidth}
        \centering
     \includegraphics[width=\linewidth, trim=0 0 0 4, clip]{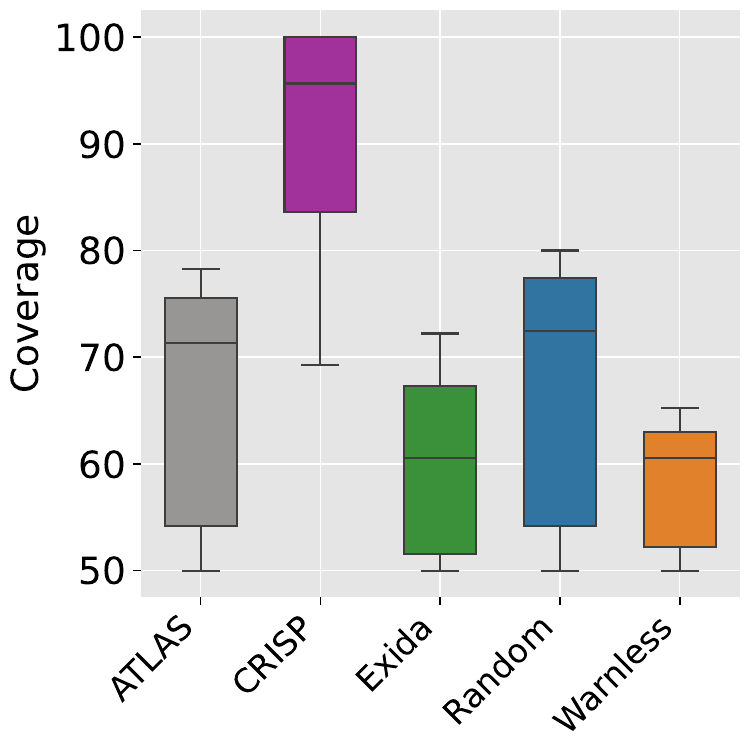}          \label{fig:sub4}
    \end{subfigure}
    \caption{Metric results \suttwo with manual \manualone and LLM \gptfivechat.}
    \label{fig:boxplots-results}
\end{figure}

\begin{figure}[p]
    \centering
    % Row 1: Run 1 and Run 2
    \begin{subfigure}[b]{0.46\linewidth}
        \centering
     \includegraphics[width=\linewidth, trim=0 65 0 10, clip]{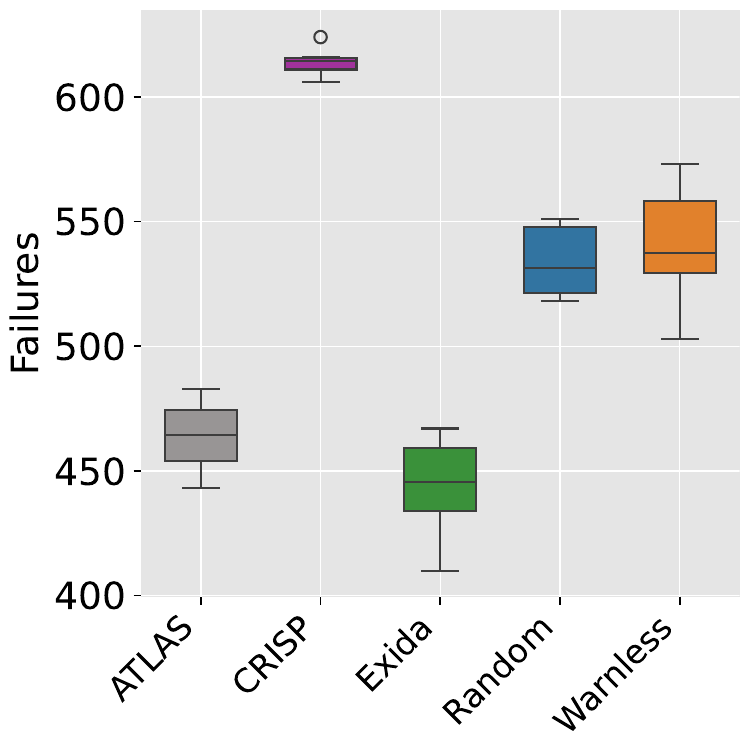}
     \label{fig:sub1}
    \end{subfigure}%
    \hspace{0.02\linewidth} % small horizontal space between figures
    \begin{subfigure}[b]{0.46\linewidth}
        \centering
     \includegraphics[width=\linewidth, trim=0 65 0 10, clip]{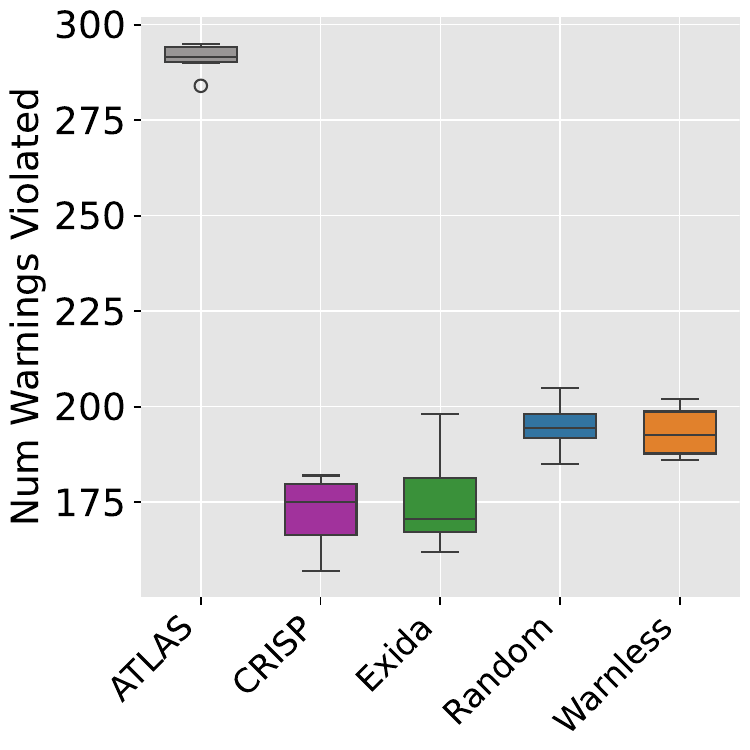}          \label{fig:sub2}
    \end{subfigure}
    \vspace{0.3cm}  % vertical space between rows
    % Row 2: Run 3 and Run 4
    \begin{subfigure}[b]{0.46\linewidth}
        \centering
        \includegraphics[width=\linewidth, trim=0 0 0 10, clip]{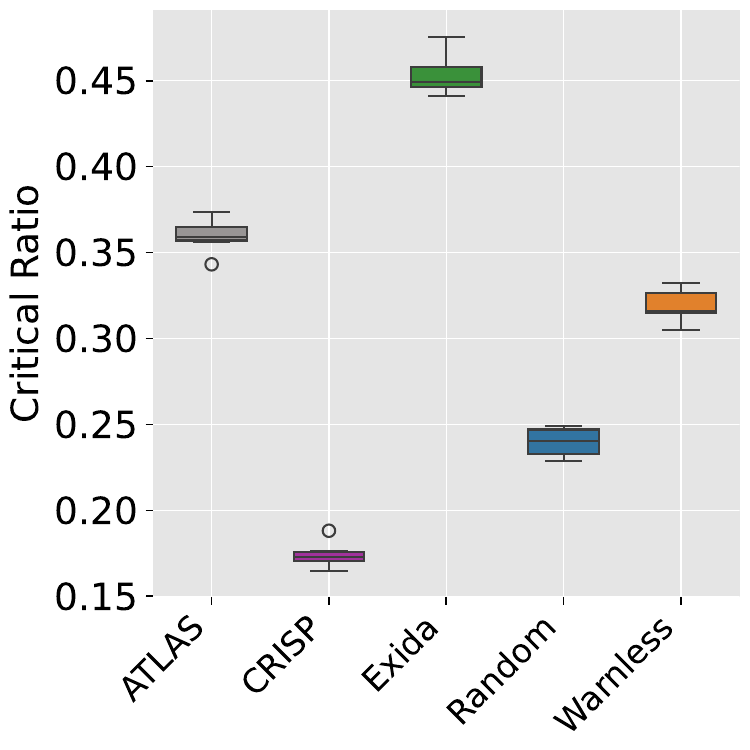}        \label{fig:sub3}
    \end{subfigure}%
    \hspace{0.02\linewidth}
    \begin{subfigure}[b]{0.46\linewidth}
        \centering
     \includegraphics[width=\linewidth, trim=0 0 0 4, clip]{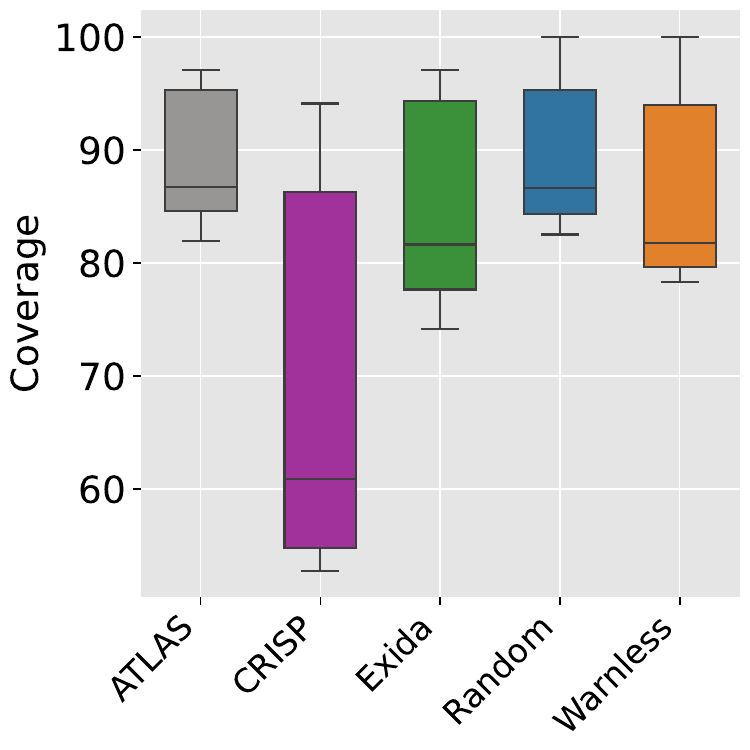}          \label{fig:sub4}
    \end{subfigure}
    \caption{Metric results \suttwo with manual \manualtwo and LLM \gptfouromini.}
    \label{fig:boxplots-results}
\end{figure}
